# Supplementary material for: A class of multi-resolution approximations for large spatial datasets
Source: arXiv:1710.08976 ancillary file (2018-07-20)
Supplement: Supplementary file 1 [file MRA_supplement.pdf]

# Supplement material to “A class of multi-resolution approximations for large spatial datasets”

Matthias Katzfuss[*][†] Wenlong Gong[*]

## 1 Additional simulation plots

We provide here additional settings for the simulation study described in Section 4 of the main document. We consider various settings for the Matérn covariance function with smoothness parameter $\nu$, range parameter $\kappa$, and noise or nugget variance $\tau^2$.

[*]Department of Statistics, Texas A&M University
[†]Corresponding author: katzfuss@gmail.com

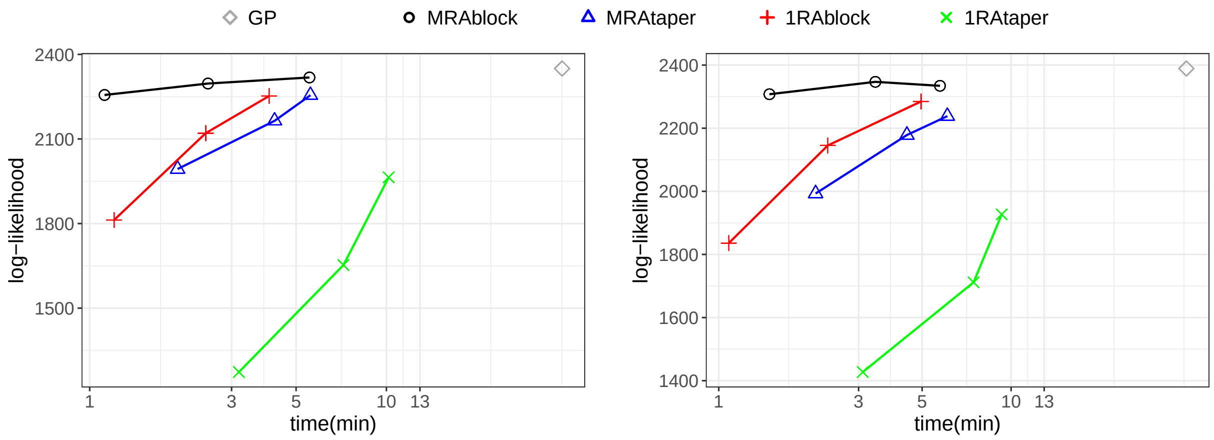


(a) $n = 32{,}786,\ \nu = 1.5,\ \kappa = 0.05,\ \tau^2 = 0.05$

(b) $n = 32{,}786,\ \nu = 2.5,\ \kappa = 0.05,\ \tau^2 = 0.05$

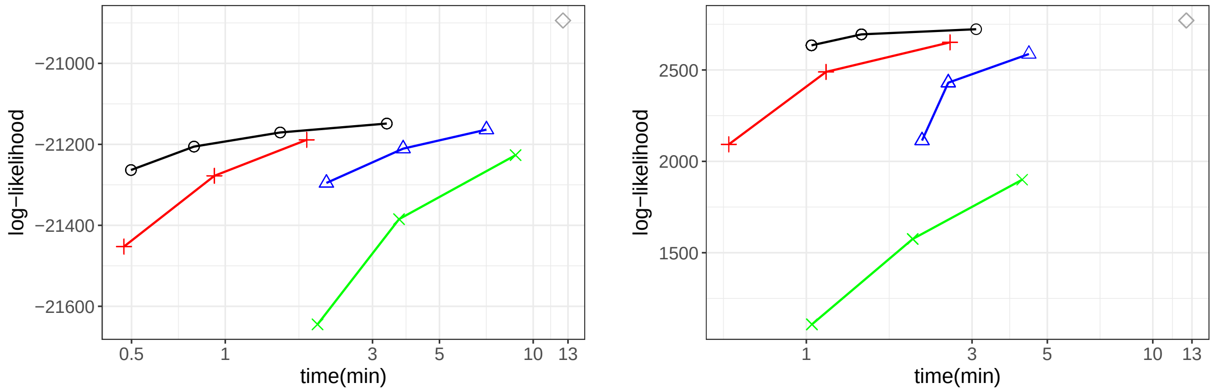


(c) $n = 32{,}786,\ \nu = 1.5,\ \kappa = 0.15,\ \tau^2 = 0.2$

(d) $n = 40{,}960,\ \nu = 1.5,\ \kappa = 0.05,\ \tau^2 = 0.05$

Figure 1: Comparison of approximation accuracy for different sample sizes in one-dimensional space

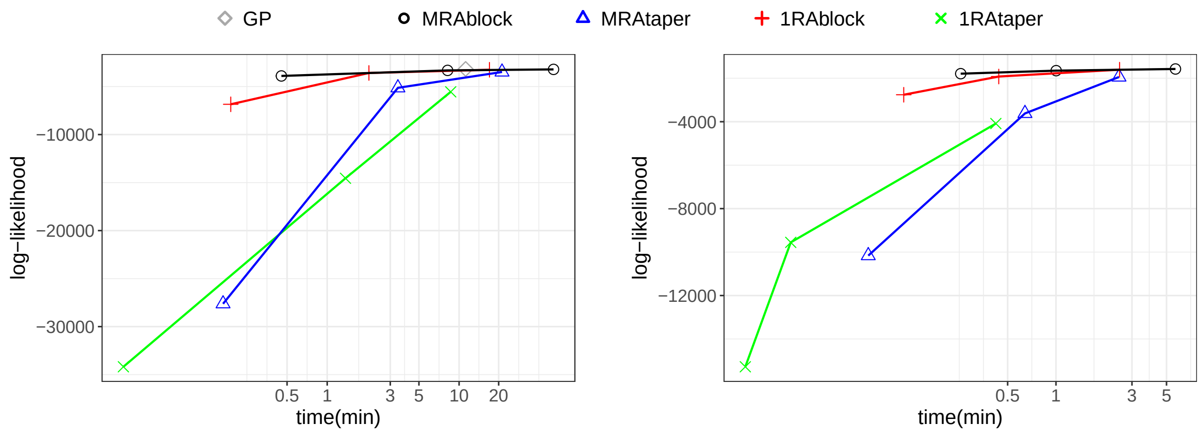


(a) $n = 25{,}600,\ \nu = 1.5,\ \kappa = 0.05,\ \tau^2 = 0.05$

(b) $n = 12{,}544,\ \nu = 2.5,\ \kappa = 0.05,\ \tau^2 = 0.05$

Figure 2: Comparison of approximation accuracy for different sample sizes in two-dimensional space
